# Supplementary material for: Learning Infinite-horizon Average-reward MDPs with Linear Function Approximation
Source: arXiv:2007.11849 source file (2021-04-26)
Supplement: Supplementary file 1 [file appendix-experiment.tex]

\section{Experiments}
\label{app: experiment}

In this section, we numerically compare the performance of our algorithm with Optimistic Q-learning \cite{wei2020model} and \politex \citep{abbasi2019politex}.

\subsection{Environmnets}
Three different environments are considered: \textit{Cartpole, LinearRiverSwim} and \textit{RandomLinearMDP}. The Cartpole environment is a continuous state space MDP with finite action. The LinearRiverSwim and the RandomLinearMDP are tabular MDPs with special structure that can be combined with function approximation. The details about these environments are provided below.

\paragraph{Cartpole.} In the Cartpole environment, the goal of the agent is to balance an inverted pole attached to a cart that can move on a frictionless rail. The original state consists of the horizontal position and velocity of the cart as well as the angular position and velocity of the tip of the pole, and we add to this state space the products of any two original features as additional features.
The agent can either push the cart to the right or left. In the finite-horizon version of Cartpole \cite{barto1983neuronlike}, each episode lasts for at most 200 steps. An episode can end earlier if the pole angle is beyond 12 degrees. The agent receives a reward of 1 for each time step that the pole is balanced. In this paper, an infinite-horizon variant of the original Cartpole environment is considered where upon terminating an episode, the agent enters a non-rewarding state under any action and can reset from there with a small probability of 0.05 at each time step. If a policy is successful to maintain the pole balanced during the 200 steps, then it will remain in the non-rewarding state for an average of 20 steps and thus enjoying $J^* = 200/220$.

\paragraph{LinearRiverSwim.} LinearRiverSwim is a tabular MDP based on the RiverSwim environment \cite{strehl2008analysis,ouyang2017learning}. The origianl RiverSwim environment, models an agent in a river that can either swim left (in the direction of the river current) or swim right. If he decides to swim left he is always successful, but if he decides to swim right, he might fail with some probability. Taking action left in the leftmost state results in a reward of 0.2 and taking action right in the rightmost state results in a reward of 1. All other states and actions have no reward. The optimal policy is to always swim right to reach the rightmost state and maximize the cumulative reward. The LinearRiverSwim is a modification of the original RiverSwim that replicates each state for 6 times (total of 36 states in 7 dimensions). At each time step, the agent might move to any of the copies of the destination state with equal probability.

\paragraph{RandomLinearMDP.} The RandomLinearMDP simulates a linear MDP with 100 states and 2 actions in 3 dimensions whose features are chosen uniformly at random. Learning this environment is much easier than LinearRiverSwim and Cartpole due to its ergodic nature.

\subsection{Details and Discussions}
\paragraph{Implementation Details.} 10 independent Monte-Carlo simulations are performed for each experiment. The hyper parameters such as the learning rate, the confidence interval of the optimistic algorithms, the estimation windows, etc., are all tuned for the best performance. For more details on hyper parameters, see Table \ref{tab: hyper parameters}.

\begin{table*}
\caption{The hyper parameters of the algorithms. All the hyper parameters are tuned for the best performance.}
\label{tab: hyper parameters}
\begin{center}

\begin{tabular}{ |c|l|l| }
\hline
 & \textbf{Algorithm} & \textbf{Parameters} \\ \hline
\multirow{2}{*}{Cartpole}
&\politex & $B = 5000$, $\eta = 0.004$, $\mu = 0$ \\
 & MDP-EXP2 & $N=500$, $B=5000$, $\eta = 0.002$, $\mu = 0$ \\ \hline
 \hline
\multirow{4}{*}{LinearRiverSwim} 
&Optimistic Q-learning & $\gamma = 0.95$, $c = 1$, $b_\tau = c \sqrt{H/\tau}$ \\
 & \politex & $B = 5000$, $\eta = 10$, $\mu = 0$ \\
&  Optimistic LSVI & $\gamma=0.99$, $\beta=1$, $\lambda=0.01$, $C=2$ \\ 
& MDP-EXP2 & $N=100$, $B=1000$, $\eta = 10$, $\mu = 0$  \\ \hline
\hline
\multirow{4}{*}{RandomLinearMDP} 
&Optimistic Q-learning & $\gamma = 0.1$, $c = 0.1$, $b_\tau = c \sqrt{H/\tau}$ \\
 & \politex & $B = 20$, $\eta = 10$, $\mu = 0$ \\
&  Optimistic LSVI & $\gamma=0.8$, $\beta=0.01$, $\lambda=0.01$, $C=2$ \\ 
& MDP-EXP2 & $N=10$, $B=100$, $\eta = 10$, $\mu = 0$ \\ \hline
\end{tabular}
\end{center}
\end{table*}

\paragraph{Discussion.} 

The three environments we test on have different properties. The experiments we conduct show that different algorithms excel in different environments. The properties of the environments can be summarized as below:  
\begin{itemize}
     \item \textbf{Cartpole}. 
     In this environment, the MDP does not have a linear transition function or a linear reward function, and we indeed observe that \algDis suffers linear regret (not plotted) since it heavily relies on the linear MDP assumption.
     On the other hand, \politex and \algExp still ensure sublinear regret.
     As discussed in \pref{sec: mdpexp2}, these algorithms only require the value function to be linear in the feature and are less vulnerable to model-misspecification.
      One can also see that our \algExp outperforms \politex, supporting our theory.
      
       \item \textbf{LinearRiverSwim}. 
       By construction, this is a linear MDP and algorithms such as \algDis and Optimistic Q-learning \cite{wei2020model} perform very well. 
       On the other hand, since the uniformly mixing assumption does not hold in this instance, \politex and \algExp both suffer linear regret.
       
       \item \textbf{RandomLinearMDP}. 
       This is a relatively easy instance where all the assumptions hold true. 
       All algorithms perform well in this case.
       In particular, Optimistic Q-learning, \algDis, and \politex even achieve negative regret sometimes.
\end{itemize}

\begin{figure}
\begin{center}
\includegraphics[scale=.45]{CartpoleEnv}
\caption{Performance comparison of our MDP-EXP2 and \politex in the Cartpole environment. }
\end{center}
\end{figure}

\begin{figure}
\begin{center}
\includegraphics[scale=.4]{LinearRiverSwimEnv}
\includegraphics[scale=.4]{RandomLinearMDPEnv}
\caption{Performance comparison of our algorithms and the benchmarks in the LinearRiverSwim and RandomLinearMDP environments.}
\end{center}
\end{figure}
